# Supplementary material for: Mitigating error cancellation in density functional approximations via machine learning correction
Source: arXiv:2504.14961 source file (2025-04-21)
Supplement: Supplementary file 1 [file SI.pdf]

**Supplemental Material for**

# Mitigating error cancellation in density functional approximations via machine learning correction

Zipeng An,[1] JingChun Wang,[2] Yapeng Zhang,[1] Zhiyu Li,[3]
Jiang Wu,[4] Yalun Zheng,[4] GuanHua Chen,[4,*] and Xiao Zheng[3,†]

[1]*Hefei National Research Center for Physical Sciences at the Microscale & Synergetic Innovation Center of Quantum Information and Quantum Physics, University of Science and Technology of China, Hefei, Anhui 230026, China*

[2]*Department of Chemistry, University of Basel, Klingelbergstrasse 80, CH-4056 Basel, Switzerland*

[3]*Department of Chemistry, Fudan University, Shanghai 200438, China*

[4]*Department of Chemistry, The University of Hong Kong, Pokfulam Road, Hong Kong, China*

(Dated: February 26, 2025)

## CONTENTS

I. Computational results in TEST12 database S2

II. Computational results in GMTKN55 database S19

References S21

# I. COMPUTATIONAL RESULTS IN TEST12 DATABASE

The reference relative energies in the TEST12 database, along with the detailed computational results obtained among B3LYP, ML-B3LYP-g and ML-B3LYP-p methods, are summarized in Tables tables S1 to S5. It should be noted that all energy values are expressed in kcal/mol.

TABLE S1: Computational results in TEST12 database, part A: AE and HOF

1. G2-AE set

| Molecule | Ref [1] | B3LYP | ML-B3LYP-g | ML-B3LYP-p |
|---|---|---|---|---|
| LiH | 57.9 | 57.7 | 57.9 | 58.1 |
| BeH | 50.8 | 56.9 | 57.2 | 54.0 |
| CH | 84.0 | 85.0 | 85.9 | 84.2 |
| $CH_2(^3B_1)$ | 190.5 | 191.4 | 192.5 | 194.1 |
| $CH_2(^1A_1)$ | 181.0 | 179.9 | 182.3 | 181.3 |
| $CH_3$ | 307.6 | 308.9 | 310.9 | 309.2 |
| $CH_4$ | 420.1 | 419.5 | 423.0 | 421.5 |
| NH | 82.9 | 87.2 | 88.0 | 83.7 |
| $NH_2$ | 182.3 | 186.4 | 188.1 | 181.7 |
| $NH_3$ | 297.8 | 298.6 | 302.0 | 296.4 |
| OH | 107.1 | 107.1 | 108.0 | 107.0 |
| $OH_2$ | 233.0 | 228.8 | 231.0 | 231.0 |
| FH | 141.7 | 138.0 | 139.2 | 141.2 |
| $SiH_2(^1A_1)$ | 153.7 | 153.3 | 154.1 | 152.1 |
| $SiH_2(^3B_1)$ | 132.8 | 132.9 | 133.4 | 130.6 |
| $SiH_3$ | 227.9 | 228.1 | 229.1 | 224.9 |
| $SiH_4$ | 324.5 | 323.2 | 324.6 | 320.2 |
| $PH_2$ | 154.3 | 158.1 | 159.6 | 153.7 |
| $PH_3$ | 241.9 | 243.9 | 245.9 | 240.7 |
| $SH_2$ | 183.7 | 181.3 | 183.6 | 184.3 |
| ClH | 107.4 | 104.6 | 106.5 | 108.4 |
| $Li_2$ | 24.2 | 20.2 | 20.3 | 18.3 |
| LiF | 139.6 | 135.2 | 136.3 | 136.6 |
| $C_2H_2$ | 405.3 | 401.0 | 405.9 | 404.7 |
| $C_2H_4$ | 563.7 | 561.2 | 566.8 | 565.0 |
| $C_2H_6$ | 712.6 | 709.1 | 715.5 | 713.9 |
| CN | 181.3 | 177.2 | 180.3 | 175.4 |
| HCN | 313.3 | 310.6 | 315.3 | 310.3 |
| CO | 259.9 | 253.2 | 256.3 | 257.0 |
| HCO | 279.5 | 278.7 | 281.3 | 278.9 |
| $H_2CO$ | 374.6 | 371.5 | 375.8 | 375.0 |

| | | | | |
|---|---|---|---|---|
| $H_3COH$ | 513.3 | 508.8 | 513.9 | 512.7 |
| $N_2$ | 228.4 | 225.6 | 230.2 | 222.7 |
| $H_2NNH_2$ | 438.0 | 440.2 | 446.4 | 435.9 |
| NO | 152.8 | 153.8 | 156.2 | 149.9 |
| $O_2$ | 120.9 | 121.4 | 122.3 | 116.8 |
| HOOH | 269.2 | 264.0 | 267.8 | 269.8 |
| $F_2$ | 38.8 | 36.1 | 37.8 | 45.6 |
| $CO_2$ | 390.5 | 384.9 | 390.1 | 390.5 |
| $Na_2$ | 17.2 | 16.9 | 16.9 | 16.4 |
| $Si_2$ | 73.6 | 74.7 | 75.0 | 70.4 |
| $P_2$ | 116.9 | 114.6 | 116.6 | 110.1 |
| $S_2$ | 103.7 | 102.7 | 104.4 | 97.3 |
| $Cl_2$ | 59.3 | 55.1 | 58.1 | 62.7 |
| NaCl | 98.7 | 92.4 | 94.0 | 97.0 |
| SiO | 193.4 | 186.0 | 187.9 | 186.9 |
| SC | 172.0 | 165.5 | 168.9 | 170.8 |
| SO | 126.4 | 124.9 | 125.9 | 121.0 |
| ClO | 64.8 | 65.1 | 66.6 | 66.3 |
| FCl | 62.7 | 59.8 | 62.2 | 66.9 |
| $Si_2H_6$ | 535.5 | 529.7 | 531.9 | 524.6 |
| $CH_3Cl$ | 395.8 | 391.3 | 396.1 | 397.4 |
| $H_3CSH$ | 475.0 | 470.0 | 475.2 | 475.5 |
| HOCl | 166.2 | 161.1 | 164.6 | 167.6 |
| $SO_2$ | 260.9 | 246.8 | 251.8 | 253.2 |
| $BF_3$ | 471.4 | 461.8 | 465.3 | 469.0 |
| $BCl_3$ | 325.0 | 312.7 | 318.5 | 325.7 |
| $AlF_3$ | 432.1 | 412.9 | 416.0 | 417.4 |
| $AlCl_3$ | 313.3 | 293.1 | 298.2 | 301.7 |
| $CF_4$ | 479.4 | 465.8 | 471.3 | 479.2 |
| $CCl_4$ | 315.2 | 294.8 | 303.1 | 314.6 |
| COS | 336.2 | 331.0 | 336.3 | 338.0 |
| $CS_2$ | 280.6 | 275.6 | 281.2 | 284.0 |
| $CF_2O$ | 421.1 | 412.9 | 418.3 | 422.5 |
| $SiF_4$ | 578.3 | 552.2 | 556.5 | 556.7 |
| $SiCl_4$ | 389.0 | 362.4 | 369.4 | 373.3 |
| $N_2O$ | 271.0 | 270.5 | 277.3 | 270.8 |
| ClNO | 192.0 | 191.0 | 196.2 | 196.5 |
| $NF_3$ | 206.4 | 205.4 | 210.5 | 215.0 |
| $PF_3$ | 365.9 | 355.4 | 359.3 | 356.7 |
| $O_3$ | 147.2 | 136.2 | 141.0 | 147.5 |
| $F_2O$ | 93.9 | 91.8 | 95.2 | 104.5 |

| | | | | |
|---|---|---|---|---|
| $ClF_3$ | 128.4 | 125.9 | 130.2 | 140.6 |
| $C_2F_4$ | 590.5 | 580.4 | 588.1 | 595.4 |
| $C_2Cl_4$ | 472.4 | 450.7 | 461.4 | 472.9 |
| $CF_3CN$ | 642.5 | 629.2 | 638.4 | 640.0 |
| $CH_3CCH$ (propyne) | 705.2 | 699.5 | 707.3 | 706.0 |
| $CH_2CCH_2$ (allene) | 703.7 | 701.7 | 709.5 | 707.9 |
| $C_3H_4$ (cyclopropene) | 681.7 | 676.0 | 683.8 | 683.9 |
| $CH_3CHCH_2$ (propylene) | 861.0 | 855.6 | 864.1 | 862.1 |
| $C_3H_6$ (cyclopropane) | 853.5 | 846.5 | 855.1 | 854.9 |
| $C_3H_8$ (propane) | 1007.2 | 999.9 | 1009.2 | 1007.4 |
| $CH_2CHCHCH_2$ (butadiene) | 1012.8 | 1006.0 | 1016.7 | 1014.2 |
| $C_4H_6$ (2-butyne) | 1004.1 | 996.7 | 1007.4 | 1005.9 |
| $C_4H_6$ (methylene cyclopropane) | 993.0 | 985.7 | 996.4 | 996.1 |
| $C_4H_6$ (bicyclobutane) | 986.0 | 974.8 | 985.6 | 986.9 |
| $C_4H_6$ (cyclobutene) | 1001.3 | 990.7 | 1001.4 | 1001.3 |
| $C_4H_8$ (cyclobutane) | 1149.9 | 1137.6 | 1149.0 | 1148.8 |
| $C_4H_8$ (isobutene) | 1159.1 | 1149.6 | 1161.0 | 1158.9 |
| $C_4H_{10}$ (*trans* butene) | 1301.9 | 1290.7 | 1302.8 | 1300.8 |
| $C_4H_{10}$ (isobutane) | 1303.3 | 1291.1 | 1303.3 | 1301.2 |
| $C_5H_8$ (spiropentane) | 1285.0 | 1271.9 | 1285.6 | 1286.7 |
| $C_6H_6$ (benzene) | 1368.9 | 1356.7 | 1371.9 | 1370.2 |
| $CH_2F_2$ | 438.1 | 432.9 | 437.5 | 439.9 |
| $CHF_3$ | 460.0 | 450.9 | 456.0 | 461.0 |
| $CH_2Cl_2$ | 371.5 | 362.6 | 368.6 | 373.2 |
| $CHCl_3$ | 345.2 | 331.1 | 338.3 | 346.3 |
| $CH_3NH_2$ (methylamine) | 581.9 | 581.1 | 587.4 | 581.0 |
| $CH_3CN$ (methyl cyanide) | 616.3 | 612.5 | 620.2 | 615.0 |
| $CH_3NO_2$ (nitromethane) | 599.4 | 598.3 | 607.4 | 603.9 |
| $CH_3ONO$ (methyl nitrite) | 601.9 | 594.4 | 603.2 | 600.0 |
| $CH_3SiH_3$ (methyl silane) | 628.9 | 623.7 | 628.0 | 623.5 |
| HCOOH (formic acid) | 502.1 | 495.4 | 501.3 | 500.9 |
| $HCOOCH_3$ (methyl formate) | 786.9 | 778.4 | 787.2 | 785.4 |
| $CH_3CONH_2$ (acetamide) | 868.5 | 863.2 | 873.3 | 867.2 |
| $C_2H_4NH$ (aziridine) | 720.1 | 716.1 | 724.6 | 719.6 |
| NCCN (cyanogen) | 501.9 | 498.1 | 507.1 | 498.3 |
| $(CH_3)_2NH$ (dimethylamine) | 870.1 | 866.6 | 875.7 | 868.5 |
| $CH_3CH_2NH_2$ (*trans* ethylamine) | 878.3 | 873.8 | 883.0 | 876.4 |
| $CH_2CO$ (ketene) | 533.5 | 530.9 | 537.3 | 537.1 |
| $C_2H_4O$ (oxirane) | 651.4 | 644.9 | 652.2 | 652.0 |
| $CH_3CHO$ (acetaldehyde) | 677.7 | 672.4 | 679.6 | 678.7 |
| HCOCOH (glyoxal) | 635.2 | 626.9 | 634.9 | 634.8 |

| | | | | |
|---|---|---|---|---|
| $CH_3CH_2OH$ (ethanol) | 810.9 | 802.9 | 810.9 | 809.4 |
| $CH_3OCH_3$ (dimethylether) | 798.6 | 792.5 | 800.5 | 798.0 |
| $C_2H_4S$ (thiooxirane) | 626.3 | 617.2 | 624.6 | 625.7 |
| $(CH_3)_2SO$ (dimethyl sulfoxide) | 857.4 | 844.0 | 853.9 | 853.9 |
| $C_2H_5SH$ (ethanethiol) | 770.1 | 761.2 | 769.3 | 769.5 |
| $CH_3SCH_3$ (dimethyl sulphide) | 769.0 | 760.5 | 768.5 | 768.6 |
| $CH_2CHF$ | 573.7 | 569.8 | 575.9 | 576.2 |
| $C_2H_5Cl$ (ethyl chloride) | 692.5 | 684.5 | 692.1 | 693.2 |
| $CH_2CHCl$ (vinyl chloride) | 544.1 | 537.6 | 544.5 | 545.9 |
| $CH_2CHCN$ (acrylonitrile) | 762.8 | 757.5 | 767.4 | 761.6 |
| $CH_3COCH_3$ (acetone) | 979.3 | 970.5 | 980.5 | 979.4 |
| $CH_3COOH$ (acetic acid) | 803.9 | 794.0 | 802.8 | 802.2 |
| $CH_3COF$ (acetyl fluoride) | 706.9 | 699.1 | 706.8 | 708.1 |
| $CH_3COCl$ (acetyl chloride) | 668.9 | 660.1 | 668.4 | 670.8 |
| $CH_3CH_2CH_2Cl$ (propyl chloride) | 987.2 | 975.2 | 985.7 | 986.6 |
| $(CH_3)_2CHOH$ (isopropanol) | 1109.2 | 1096.7 | 1107.5 | 1105.8 |
| $C_2H_5OCH_3$ (methyl ethyl ether) | 1096.3 | 1086.5 | 1097.4 | 1094.7 |
| $(CH_3)_3N$ (trimethylamine) | 1161.1 | 1153.5 | 1165.5 | 1157.4 |
| $C_4H_4O$ (furan) | 995.3 | 983.6 | 995.3 | 994.4 |
| $C_4H_4S$ (thiophene) | 965.2 | 950.5 | 962.3 | 964.2 |
| $C_4H_5N$ (pyrrole) | 1072.9 | 1064.6 | 1077.5 | 1071.6 |
| $C_5H_5N$ (pyridine) | 1239.0 | 1230.6 | 1245.7 | 1239.1 |
| $H_2$ | 109.4 | 110.0 | 110.6 | 109.9 |
| HS | 87.6 | 87.8 | 89.0 | 88.0 |
| CCH | 265.8 | 261.0 | 264.5 | 265.6 |
| $C_2H_3(^2A')$ | 445.7 | 445.5 | 449.8 | 448.0 |
| $CH_3CO(^2A')$ | 582.4 | 579.7 | 585.0 | 582.9 |
| $H_2COH(^2A)$ | 410.0 | 408.3 | 411.8 | 410.4 |
| $CH_3O(^2A')$ | 400.2 | 401.8 | 405.5 | 402.7 |
| $CH_3CH_2O(^2A")$ | 697.7 | 692.5 | 699.1 | 696.4 |
| $CH_3S(^2A')$ | 382.6 | 380.9 | 384.9 | 383.8 |
| $C_2H_5(^2A')$ | 603.7 | 603.1 | 608.0 | 606.3 |
| $(CH_3)_2CH(^2A')$ | 901.0 | 897.6 | 905.5 | 903.8 |
| $(CH_3)_3C$ (*t*-butyl radical) | 1199.0 | 1191.9 | 1202.7 | 1201.0 |
| $NO_2$ | 228.0 | 229.7 | 233.9 | 229.5 |
| MAD | | 6.1 | 3.2 | 2.6 |

2. G3-HOF set

| Molecule | Ref [2] | B3LYP | ML-B3LYP-g | ML-B3LYP-p |
|---|---|---|---|---|
| $CH_3CHCCH_2$ (methyl allene) | 38.8 | 42.3 | 31.7 | 33.5 |
| $C_5H_8$ (isoprene) | 18.0 | 27.5 | 13.9 | 16.6 |

| | | | | |
|---|---|---|---|---|
| $C_5H_{10}$ (cyclopentane) | -18.3 | -3.7 | -18.1 | -17.7 |
| $C_5H_{12}$ (*n*-pentane) | -35.1 | -23.4 | -38.4 | -36.2 |
| $C_5H_{12}$ (neopentane) | -40.2 | -24.2 | -39.2 | -36.8 |
| $C_6H_8$ (1,3 cyclohexadiene) | 25.4 | 40.1 | 24.3 | 25.3 |
| $C_6H_8$ (1,4 cyclohexadiene) | 25.0 | 39.8 | 24.0 | 24.9 |
| $C_6H_{12}$ (cyclohexane) | -29.5 | -9.9 | -27.2 | -26.4 |
| $C_6H_{14}$ (*n*-hexane) | -39.9 | -25.0 | -42.9 | -40.5 |
| $C_6H_{14}$ (3-methyl pentane) | -41.1 | -23.5 | -41.4 | -39.0 |
| $C_6H_5CH_3$ (toluene) | 12.0 | 24.8 | 6.7 | 8.4 |
| $C_7H_{16}$ (*n*-heptane) | -44.9 | -27.1 | -47.9 | -45.3 |
| $C_8H_8$ (cyclooctatetraene) | 70.7 | 89.3 | 69.3 | 71.2 |
| $C_8H_{18}$ (*n*-octane) | -49.9 | -28.7 | -52.4 | -49.7 |
| $C_{10}H_8$ (naphthalene) | 35.9 | 55.3 | 30.6 | 31.9 |
| $C_{10}H_8$ (azulene) | 69.1 | 88.5 | 63.9 | 64.8 |
| $CH_3COOCH_3$ (methyl acetate) | -98.4 | -89.4 | -101.1 | -99.0 |
| $(CH_3)_3COH$ (*t*-butanol) | -74.7 | -59.2 | -73.0 | -71.0 |
| $C_6H_5NH_2$ (aniline) | 20.8 | 30.3 | 12.3 | 18.7 |
| $C_6H_5OH$ (phenol) | -23.0 | -9.3 | -26.1 | -25.0 |
| $C_4H_6O$ (divinyl ether) | -3.3 | 3.4 | -8.9 | -6.0 |
| $C_4H_8O$ (tetrahydrofuran) | -44.0 | -30.5 | -43.7 | -42.5 |
| $C_5H_8O$ (cyclopentanone) | -45.9 | -31.0 | -46.2 | -46.6 |
| $C_6H_4O_2$ (benzoquinone) | -29.4 | -12.4 | -29.9 | -29.8 |
| $C_4H_4N_2$ (pyrimidine) | 46.8 | 47.6 | 32.6 | 44.0 |
| $C_2H_6O_2S$ (dimethyl sulphone) | -89.2 | -71.1 | -82.9 | -82.4 |
| $C_6H_5Cl$ (chlorobenzene) | 12.4 | 25.9 | 9.4 | 7.9 |
| $NCCH_2CH_2CN$ (1,2-dicyano ethane) | 50.1 | 59.8 | 45.0 | 54.3 |
| $C_4H_4N_2$ (pyrazine) | 46.9 | 51.7 | 36.7 | 48.0 |
| $CH_3COCCH$ (acetyl acetylene) | 15.6 | 26.9 | 15.5 | 16.4 |
| $CH_3CHCHCHO$ (crotonaldehyde) | -24.0 | -17.7 | -29.9 | -28.4 |
| $CH_3COOCOCH_3$ (acetic anhydride) | -136.8 | -124.6 | -139.9 | -139.0 |
| $C_4H_6S$ (2,5-dihydrothiophene) | 20.8 | 33.5 | 21.1 | 19.8 |
| $(CH_3)_2CHCN$ (isobutane nitrile) | 5.6 | 17.0 | 3.6 | 9.3 |
| $CH_3COCH_2CH_3$ (methyl ethyl ketone) | -57.1 | -47.3 | -60.2 | -58.9 |
| $(CH_3)_2CHCHO$ (isobutanal) | -51.6 | -39.2 | -52.1 | -50.9 |
| $C_4H_8O_2$ (1,4-dioxane) | -75.5 | -59.8 | -74.5 | -72.4 |
| $C_4H_8S$ (tetrahydrothiophene) | -8.2 | 8.1 | -5.1 | -6.5 |
| $(CH_3)_3CCl$ (*t*-butyl chloride) | -43.5 | -28.0 | -41.4 | -41.8 |
| $CH_3CH_2CH_2CH_2Cl$ (*n*-butyl chloride) | -37.0 | -24.6 | -38.0 | -38.3 |
| $C_4H_8NH$ (tetrahydropyrrole) | -0.8 | 9.9 | -4.3 | 1.5 |
| $CH_3CH_2CH(CH_3)NO_2$ (nitro-*s*-butane) | -39.1 | -25.0 | -42.7 | -38.6 |
| $CH_3CH_2OCH_2CH_3$ (diethyl ether) | -60.3 | -50.2 | -64.0 | -61.0 |

| | | | | |
|---|---|---|---|---|
| $CH_3CH(OCH_3)_2$ (1,1-dimethoxy ethane) | -93.1 | -78.2 | -93.5 | -89.7 |
| $(CH_3)_3CSH$ ($t$-butanethiol) | -26.2 | -9.6 | -23.4 | -23.0 |
| $CH_3CH_2SSCH_2CH_3$ (diethyl disulfide) | -17.9 | -1.7 | -17.3 | -18.1 |
| $(CH_3)_3CNH_2$ ($t$-butylamine) | -28.9 | -15.9 | -30.8 | -23.7 |
| $Si(CH_3)_4$ (tetramethylsilane) | -55.7 | -37.7 | -50.7 | -45.8 |
| $C_5H_6S$ (2-methyl thiophene) | 20.0 | 34.1 | 19.4 | 17.7 |
| $C_5H_7N$ (N-methyl pyrrole) | 24.6 | 32.9 | 17.1 | 23.9 |
| $C_5H_{10}O$ (tetrahydropyran) | -53.4 | -35.5 | -51.6 | -50.1 |
| $CH_3CH_2COCH_2CH_3$ (diethyl ketone) | -61.6 | -49.4 | -65.2 | -63.7 |
| $CH_3COOCH(CH_3)_2$ (isopropyl acetate) | -115.1 | -98.4 | -115.9 | -113.3 |
| $C_5H_{10}S$ (tetrahydrothiopyran) | -15.2 | 5.1 | -11 | -12.1 |
| cyc$-C_5H_{10}NH$ (piperidine) | -11.3 | 5.0 | -12.2 | -6.1 |
| $(CH_3)_3COCH_3$ ($t$-butyl methyl ether) | -67.8 | -50.5 | -67.1 | -63.8 |
| $C_6H_4F_2$ (1,3-difluorobenzene) | -73.9 | -61.9 | -78.2 | -80.8 |
| $C_6H_4F_2$ (1,4-difluorobenzene) | -73.3 | -61.3 | -77.6 | -80.1 |
| $C_6H_5F$ (fluorobenzene) | -27.7 | -16.6 | -32.4 | -32.8 |
| $(CH_3)_2CHOCH(CH_3)_2$ (di-isopropyl ether) | -76.3 | -56.8 | -76.3 | -72.8 |
| $PF_5$ | -381.4 | -359.6 | -365.7 | -364.9 |
| $SF_6$ | -291.7 | -267.0 | -274.6 | -285.5 |
| $P_4$ | 14.1 | 25.4 | 21.0 | 39.0 |
| $SO_3$ | -94.6 | -78.8 | -85.7 | -87.6 |
| $SCl_2$ | -4.2 | 0.7 | -4.1 | -9.2 |
| $POCl_3$ | -133.8 | -116.9 | -124.7 | -125.0 |
| $PCl_5$ | -86.1 | -66.6 | -75.9 | -80.0 |
| $Cl_2O_2S$ | -84.8 | -66.7 | -75.1 | -81.2 |
| $PCl_3$ | -69.0 | -60.6 | -66.5 | -67.1 |
| $Cl_2S_2$ | -4.0 | -0.1 | -6.6 | -13.1 |
| $SiCl_2$ | -40.3 | -33.8 | -37.2 | -38.6 |
| $CF_3Cl$ | -169.5 | -159.5 | -165.8 | -174.6 |
| $C_2F_6$ | -321.3 | -303.8 | -313.3 | -324.9 |
| $CF_3$ | -111.3 | -109.3 | -112.7 | -119.0 |
| $C_6H_5$ (phenyl radical) | 81.2 | 90.3 | 76.4 | 78.6 |
| MAD | | 13.5 | 3.8 | 3.6 |

3. P6-AE set

| Molecule | Ref [3] | B3LYP | ML-B3LYP-g | ML-B3LYP-p |
|---|---|---|---|---|
| $C_4H_4$ | 793.9 | 783.5 | 793.7 | 796.4 |
| $C_6H_6$ | 1254.3 | 1231.2 | 1246.3 | 1251.0 |
| $C_8H_8$ | 1706.6 | 1670.8 | 1690.8 | 1697.3 |
| $C_{10}H_{10}$ | 2196.5 | 2147.6 | 2172.8 | 2180.7 |
| $C_{12}H_{12}$ | 2718.3 | 2654.4 | 2685.1 | 2693.8 |

| | | | | |
|---|---|---|---|---|
| $C_{20}H_{20}$ | 4621.5 | 4505.5 | 4556.6 | 4570.8 |
| MAD | | 49.7 | 23.3 | 17.7 |

4. AlkAtom19-AE set

| Molecule | Ref [3] | B3LYP | ML-B3LYP-g | ML-B3LYP-p |
|---|---|---|---|---|
| methane | 420.4 | 419.5 | 423.0 | 421.5 |
| ethane | 713.1 | 709.1 | 715.5 | 713.8 |
| propane | 1007.9 | 999.9 | 1009.2 | 1007.3 |
| butane | 1302.9 | 1290.7 | 1302.9 | 1300.8 |
| pentane | 1597.8 | 1581.4 | 1596.4 | 1594.1 |
| hexane | 1892.7 | 1872.1 | 1890.0 | 1887.5 |
| heptane | 2187.7 | 2162.8 | 2183.6 | 2180.9 |
| octane | 2482.6 | 2453.5 | 2477.2 | 2474.3 |
| isobutane | 1304.3 | 1291.2 | 1303.3 | 1301.2 |
| isopentane | 1598.7 | 1580.9 | 1596.0 | 1593.7 |
| isohexane | 1893.6 | 1871.5 | 1889.5 | 1887.0 |
| isoheptane | 2188.6 | 2162.3 | 2183.0 | 2180.3 |
| isooctane | 2484.3 | 2449.3 | 2473.0 | 2470.0 |
| neopentane | 1601.5 | 1582.1 | 1597.1 | 1594.8 |
| neohexane | 1895.2 | 1870.7 | 1888.6 | 1886.1 |
| neoheptane | 2190.1 | 2161.2 | 2182.0 | 2179.3 |
| 3-methylpentane | 1893.0 | 1870.5 | 1888.4 | 1885.9 |
| diisopropyl | 1893.8 | 1870.0 | 1887.9 | 1885.4 |
| hexamethylethane | 2484.0 | 2445.4 | 2469.0 | 2466.0 |
| MAD | | 20.4 | 4.7 | 6.6 |

TABLE S2: Computational results in TEST12 database, part B: IP and EA

1. G2-IP set

| Molecule | Ref [4] | B3LYP | ML-B3LYP-g | ML-B3LYP-p |
|---|---|---|---|---|
| Li | 124.3 | 127.9 | 127.9 | 130.2 |
| Be | 214.9 | 208.1 | 208.2 | 211.5 |
| B | 191.4 | 199.5 | 199.4 | 200.5 |
| C | 259.7 | 264.1 | 263.9 | 267.0 |
| N | 335.3 | 335.9 | 335.8 | 340.3 |
| O | 313.9 | 323.3 | 323.7 | 321.4 |
| F | 401.7 | 406.2 | 406.8 | 408.2 |
| Na | 291.0 | 291.6 | 293.0 | 295.4 |
| Mg | 234.8 | 233.3 | 234.9 | 237.8 |
| Al | 300.0 | 302.9 | 303.6 | 303.6 |

| | | | | |
|---|---|---|---|---|
| Si | 291.0 | 289.7 | 291.0 | 293.3 |
| P | 369.9 | 369.5 | 370.6 | 373.4 |
| S | 118.5 | 122.9 | 122.9 | 123.1 |
| Cl | 176.4 | 176.7 | 176.7 | 179.3 |
| $CH_4$ | 137.9 | 136.8 | 136.8 | 138.2 |
| $NH_3$ | 187.9 | 185.2 | 185.3 | 189.7 |
| OH | 241.9 | 237.5 | 237.6 | 244.9 |
| $OH_2$ | 238.9 | 241.2 | 242.1 | 240.9 |
| FH | 299.1 | 299.2 | 300.5 | 300.6 |
| $SiH_4$ | 253.7 | 251.5 | 251.8 | 254.0 |
| PH | 234.1 | 232.5 | 232.5 | 238.0 |
| $PH_2$ | 226.5 | 226.9 | 226.8 | 229.6 |
| $PH_3$ | 227.6 | 224.6 | 224.9 | 228.5 |
| SH | 239.1 | 239.3 | 240.4 | 241.5 |
| $SH_2(^2B_1)$ | 241.4 | 238.3 | 239.3 | 243.5 |
| ClH | 294.0 | 291.9 | 293.7 | 296.9 |
| $C_2H_2$ | 262.9 | 257.2 | 258.9 | 262.7 |
| $C_2H_4$ | 242.4 | 237.4 | 238.9 | 243.1 |
| CO | 323.1 | 323.6 | 324.4 | 325.3 |
| $N_2(^2\Sigma)$ | 359.3 | 362.9 | 364.4 | 367.3 |
| $N_2(^2\Pi)$ | 385.1 | 372.6 | 374.3 | 376.3 |
| $O_2$ | 278.3 | 293.1 | 292.4 | 285.7 |
| $P_2$ | 242.8 | 235.5 | 235.8 | 242.0 |
| $S_2$ | 215.9 | 218.9 | 218.3 | 218.2 |
| $Cl_2$ | 265.2 | 260.1 | 262.5 | 269.2 |
| FCl | 292.0 | 288.2 | 290.1 | 294.1 |
| SC | 261.3 | 261.5 | 262.5 | 264.9 |
| H | 313.6 | 313.0 | 313.0 | 313.7 |
| He | 567.1 | 572.7 | 573.4 | 571.6 |
| Ne | 497.2 | 498.3 | 499.2 | 511.4 |
| Ar | 363.4 | 362.2 | 364.2 | 366.3 |
| $BF_3$ | 358.8 | 355.1 | 356.3 | 358.5 |
| $BCl_3$ | 267.5 | 257.0 | 259.6 | 266.5 |
| $B_2F_4$ | 278.3 | 264.2 | 265.3 | 267.1 |
| $CO_2$ | 317.5 | 315.2 | 316.8 | 320.9 |
| $CF_2$ | 263.4 | 258.6 | 259.8 | 261.4 |
| OCS | 257.6 | 256.2 | 257.6 | 261.4 |
| $CS_2$ | 232.2 | 229.6 | 230.5 | 238.4 |
| $CH_2$ | 239.8 | 226.8 | 227.8 | 230.7 |
| $CH_3$ | 226.9 | 226.4 | 225.7 | 228.3 |
| $C_2H_5$ | 187.3 | 186.7 | 186.0 | 187.5 |

| | | | | |
|---|---|---|---|---|
| $C_3H_4$ (cyclopropene) | 223.0 | 217.0 | 218.6 | 224.6 |
| sec-$C_3H_7$ | 170.0 | 167.7 | 166.9 | 169.3 |
| $C_6H_6$ | 213.3 | 208.2 | 209.8 | 216.0 |
| $C_6H_5CH_3$ | 203.6 | 197.6 | 199.3 | 206.0 |
| CN | 313.6 | 346.7 | 345.8 | 344.8 |
| CHO | 187.7 | 192.3 | 191.5 | 190.4 |
| $CH_2OH$ | 174.1 | 173.1 | 172.2 | 174.0 |
| $CH_3O$ | 247.4 | 243.6 | 244.7 | 250.8 |
| $CH_3OH$ | 250.2 | 245.3 | 246.8 | 251.9 |
| $CH_3F$ | 287.6 | 287.8 | 289.3 | 293.2 |
| $CH_2S$ | 216.3 | 212.4 | 213.4 | 218.1 |
| $CH_2SH$ | 173.9 | 172.4 | 171.5 | 172.0 |
| $CH_3SH$ | 217.7 | 213.6 | 214.7 | 218.7 |
| $CH_3Cl$ | 258.7 | 256.3 | 258.3 | 262.6 |
| $C_2H_5OH$ | 241.4 | 232.3 | 234.2 | 238.9 |
| $CH_3CHO$ | 235.9 | 231.6 | 233.0 | 237.5 |
| $CH_3OF$ | 261.5 | 256.8 | 258.3 | 262.7 |
| $C_2H_4S$ (thiirane) | 208.7 | 204.2 | 205.3 | 209.1 |
| $C_4H_4O$ (furan) | 203.6 | 199.3 | 200.9 | 206.3 |
| $C_2H_5OH$ | 196.2 | 190.2 | 191.9 | 199.0 |
| $C_6H_5NH_2$ (aniline) | 178.0 | 171.5 | 173.4 | 182.1 |
| $B_2H_4$ | 223.7 | 216.8 | 217.2 | 221.6 |
| NH | 311.1 | 313.6 | 313.4 | 315.5 |
| $NH_2$ | 256.9 | 259.9 | 260.8 | 260.0 |
| $N_2H_2$ | 221.2 | 218.8 | 220.6 | 226.3 |
| $N_2H_3$ | 175.5 | 178.1 | 176.7 | 174.7 |
| HOF | 293.1 | 289.5 | 291.0 | 295.2 |
| $SiH_2$ | 211.0 | 206.2 | 206.5 | 210.6 |
| $SiH_3$ | 187.7 | 186.1 | 186.1 | 188.1 |
| $Si_2H_2$ | 189.1 | 183.3 | 183.5 | 188.2 |
| $Si_2H_4$ | 186.6 | 179.7 | 179.8 | 184.5 |
| $Si_2H_5$ | 175.3 | 174.6 | 174.6 | 176.1 |
| $Si_2H_6$ | 224.6 | 218.6 | 218.8 | 224.8 |
| MAD | | 4.3 | 3.8 | 3.4 |

2. G2-EA set

| Molecule | Ref [4] | B3LYP | ML-B3LYP-g | ML-B3LYP-p |
|---|---|---|---|---|
| C | 29.1 | 22.6 | 22.5 | 30.3 |
| O | 33.7 | 36.5 | 37.1 | 39.0 |
| F | 78.4 | 79.3 | 80.3 | 84.0 |
| Si | 32.1 | 23.3 | 23.3 | 25.1 |

| | | | | |
|---|---|---|---|---|
| P | 17.3 | 11.3 | 12.0 | 11.4 |
| S | 48.0 | 48.7 | 49.7 | 51.5 |
| Cl | 83.5 | 82.7 | 84.3 | 88.4 |
| CH | 28.6 | 24.3 | 24.0 | 29.8 |
| $CH_2$ | 15.0 | 22.7 | 21.9 | 25.2 |
| $CH_3$ | 1.8 | -5.0 | -4.2 | 0.4 |
| NH | 8.8 | 2.4 | 3.0 | 4.3 |
| $NH_2$ | 17.8 | 10.4 | 11.7 | 15.9 |
| OH | 42.2 | 40.4 | 41.5 | 45.2 |
| SiH | 29.5 | 22.8 | 22.8 | 24.7 |
| $SiH_2$ | 25.8 | 21.8 | 21.7 | 23.0 |
| $SiH_3$ | 32.5 | 28.1 | 28.1 | 32.7 |
| PH | 23.8 | 16.3 | 16.7 | 19.0 |
| $PH_2$ | 29.3 | 21.3 | 21.5 | 26.6 |
| HS | 54.4 | 51.8 | 52.6 | 57.4 |
| $O_2$ | 10.1 | 10.6 | 11.5 | 18.5 |
| NO | 0.5 | 2.3 | 1.5 | 1.3 |
| CN | 89.0 | 90.2 | 91.3 | 94.6 |
| PO | 25.1 | 25.4 | 25.1 | 27.4 |
| $S_2$ | 38.3 | 36.4 | 37.5 | 43.8 |
| $Cl_2$ | 55.1 | 62.5 | 60.3 | 56.1 |
| Li | 14.3 | 6.5 | 6.5 | 6.4 |
| B | 6.5 | 2.2 | 2.3 | 7.7 |
| Na | 12.7 | 10.0 | 10.0 | 10.4 |
| Al | 10.1 | -0.5 | -0.5 | -1.5 |
| $C_2$ | 75.4 | 96.7 | 95.9 | 94.7 |
| $C_2O$ | 52.8 | 50.3 | 51.5 | 54.3 |
| $CF_2$ | 4.2 | 6.7 | 5.8 | 7.1 |
| NCO | 83.3 | 78.7 | 80.5 | 85.0 |
| $NO_2$ | 52.3 | 48.6 | 50.2 | 54.8 |
| $O_3$ | 48.4 | 60.9 | 59.5 | 56.3 |
| OF | 52.3 | 50.6 | 51.8 | 55.5 |
| $SO_2$ | 25.6 | 30.7 | 29.5 | 29.1 |
| $S_2O$ | 43.4 | 47.2 | 46.3 | 43.4 |
| $C_2H$ | 68.5 | 67.9 | 68.7 | 70.6 |
| $C_2H_3$ | 15.5 | 11.4 | 12.2 | 16.7 |
| $CH_2CC$ | 41.3 | 41.0 | 39.9 | 40.4 |
| $CH_2CCH$ | 20.5 | 18.9 | 20.1 | 26.7 |
| $CH_2CHCH_2$ | 10.8 | 6.0 | 7.3 | 13.3 |
| HCO | 7.1 | 2.7 | 3.8 | 9.8 |
| HCF | 12.5 | 13.3 | 12.4 | 14.4 |

| | | | | |
|---|---|---|---|---|
| $CH_3O$ | 36.2 | 32.2 | 33.3 | 38.3 |
| $CH_3S$ | 43.1 | 40.0 | 40.8 | 45.3 |
| $CH_2S$ | 10.8 | 11.4 | 10.4 | 9.9 |
| $CH_2CN$ | 35.5 | 32.1 | 33.6 | 39.2 |
| $CH_2NC$ | 24.4 | 21.6 | 22.8 | 28.7 |
| CHCO | 54.2 | 49.1 | 50.6 | 55.4 |
| $CH_2CHO$ | 42.0 | 39.8 | 41.2 | 45.4 |
| $CH_3CO$ | 9.7 | 3.7 | 4.9 | 9.8 |
| $CH_3CH_2O$ | 39.4 | 38.7 | 39.7 | 44.3 |
| $CH_3CH_2S$ | 45.0 | 41.6 | 42.4 | 46.6 |
| LiH | 7.8 | 4.1 | 4.1 | 4.0 |
| HNO | 7.8 | 12.1 | 10.6 | 8.6 |
| $HO_2$(HOO $^2$A") | 24.9 | 20.7 | 22.1 | 26.9 |
| MAD | | 4.3 | 3.7 | 3.7 |

TABLE S3: Computational results in TEST12 database, part C: ISO

1. ISO-C set

| Product | Reactant | Ref [3] | B3LYP | ML-B3LYP-g | ML-B3LYP-p |
|---|---|---|---|---|---|
| $C_{20}$ Cage-D2h | $C_{20}$ Bowl-C5v | 8.9 | 42.8 | 42.6 | 31.0 |
| $C_{20}$ Cage-D3h | $C_{20}$ Bowl-C5v | 8.4 | 42.7 | 42.5 | 31.0 |
| $C_{20}$ Ring-C10h | $C_{20}$ Bowl-C5v | 46.3 | -19.6 | -19.6 | -7.0 |
| $C_{24}$ Cage-Oh | $C_{24}$ Corona-D6h | 31.2 | 65.6 | 65.5 | 52.8 |
| $C_{24}$ Cage-D3d | $C_{24}$ Corona-D6h | -5.3 | 39.6 | 39.4 | 26.1 |
| $C_{24}$ Ring-C12h | $C_{24}$ Corona-D6h | 84.5 | 4.4 | 4.4 | 18.7 |
| MAD | | | 20.4 | 4.7 | 6.6 |

2. ISO20 set

| Product | Reactant | Ref [3] | B3LYP | ML-B3LYP-g | ML-B3LYP-p |
|---|---|---|---|---|---|
| OClO | ClOO | -1.7 | 2.7 | 2.7 | 3.7 |
| t-HONO | c-HONO | -0.4 | -0.7 | -0.7 | -0.8 |
| HCN | HNC | -15.2 | -14.1 | -14.3 | -14.0 |
| HNCO | HOCN | -24.7 | -28.9 | -28.9 | -28.5 |
| HNCO | HONC | -84.6 | -87.4 | -87.6 | -86.3 |
| HNCO | HCNO | -69.8 | -68.4 | -68.1 | -67.6 |
| HOCN | HONC | -59.9 | -58.5 | -58.8 | -57.8 |
| HOCN | HCNO | -45.1 | -39.5 | -39.2 | -39.1 |
| HCNO | HONC | -14.8 | -19.0 | -19.5 | -18.7 |
| $H_2CO$ | t-HCOH | -52.2 | -53.0 | -53.3 | -52.7 |
| t-HCOH | c-HCOH | -4.8 | -4.7 | -4.7 | -4.6 |

| | | | | | |
|---|---|---|---|---|---|
| $C_2H_2$ | $CH_2C$ | -45.6 | -43.1 | -43.5 | -42.8 |
| t-HOOO | c-HOOO | -0.2 | -0.1 | -0.2 | -0.2 |
| t-$N_2H_2$ | c-$N_2H_2$ | -5.4 | -5.4 | -5.4 | -5.4 |
| propyne | allene | -1.5 | 1.9 | 1.9 | 1.8 |
| formic | dioxirane | -91.9 | -92.7 | -92.5 | -89.7 |
| ketene | oxirene | -77.4 | -81.4 | -81.2 | -79.9 |
| acetaldehyde | oxirane | -26.3 | -27.8 | -27.6 | -26.9 |
| $H_2CN$ | HCNH | -7.5 | -7.8 | -7.9 | -8.1 |
| $CH_2NH_2$ | $CH_3NH$ | -7.6 | -7.1 | -7.0 | -6.5 |
| MAD | | | 2.0 | 2.0 | 2.0 |

TABLE S4: Computational results in TEST12 database, part D: BDE

1. BDE42 set

| Species | Radical 1 | Radical 2 | Ref [5] | B3LYP | ML-B3LYP-g | ML-B3LYP-p |
|---|---|---|---|---|---|---|
| $C_2H_6O$ | $OH\cdot$ | $C_2H_5\cdot$ | 94.0 | 92.7 | 94.8 | 96.0 |
| $C_2H_6$ | $CH_3\cdot$ | $CH_3\cdot$ | 90.2 | 91.4 | 93.6 | 95.3 |
| $CH_3NO_2$ | $NO_2\cdot$ | $CH_3\cdot$ | 60.8 | 78.5 | 81.5 | 83.1 |
| $C_5H_{12}O$ | $C_2H_5O\cdot$ | $C_3H_7\cdot$ | 84.8 | 85.2 | 87.4 | 88.9 |
| $C_8H_{10}$ | $CH_3\cdot$ | $C_7H_7\cdot$ | 76.4 | 74.9 | 77.7 | 82.0 |
| $C_3H_8$ | $CH_3\cdot$ | $C_2H_5\cdot$ | 88.5 | 88.0 | 90.2 | 91.8 |
| $C_4H_{10}$ | $CH_3\cdot$ | $nC_3H_7\cdot$ | 88.9 | 88.0 | 90.3 | 91.8 |
| $C_4H_{10}$ | $CH_3\cdot$ | $iC_3H_7\cdot$ | 88.2 | 84.6 | 86.8 | 88.2 |
| $C_5H_{12}$ | $CH_3\cdot$ | $C_4H_9\cdot$ | 88.8 | 88.0 | 90.2 | 91.5 |
| $C_4H_{10}$ | $C_2H_5\cdot$ | $C_2H_5\cdot$ | 86.8 | 84.5 | 86.7 | 88.2 |
| $C_5H_{12}$ | $C_2H_5\cdot$ | $nC_3H_7\cdot$ | 87.3 | 84.5 | 86.7 | 88.1 |
| $C_5H_{12}$ | $C_2H_5\cdot$ | $iC_3H_7\cdot$ | 86.1 | 80.1 | 82.3 | 83.6 |
| $C_6H_{14}$ | $C_2H_5\cdot$ | $C_4H_9\cdot$ | 86.9 | 84.4 | 86.6 | 87.9 |
| $C_3H_4$ | $CH_3\cdot$ | $C_2H\cdot$ | 126.0 | 130.0 | 132.5 | 131.3 |
| $C_4H_6$ | $C_2H_5\cdot$ | $C_2H\cdot$ | 124.0 | 126.3 | 128.7 | 127.4 |
| $CH_{40}$ | $OH\cdot$ | $CH_3\cdot$ | 92.0 | 92.9 | 95.1 | 96.4 |
| $C_3H_8O$ | $OH\cdot$ | $nC_3H_7\cdot$ | 94.2 | 92.6 | 94.8 | 95.9 |
| $C_3H_8O$ | $OH\cdot$ | $iC_3H_7\cdot$ | 95.6 | 91.7 | 93.9 | 94.9 |
| $C_4H_{10}O$ | $OH\cdot$ | $C_4H_9\cdot$ | 93.7 | 92.5 | 94.7 | 95.6 |
| $C_5H_{12}O$ | $OH\cdot$ | $C_5H_{11}\cdot$ | 95.7 | 90.3 | 92.4 | 93.0 |
| $C_2H_6O$ | $CH_3O\cdot$ | $CH_3\cdot$ | 83.2 | 81.8 | 84.0 | 86.0 |
| $C_3H_8O$ | $CH_3O\cdot$ | $C_2H_5\cdot$ | 84.2 | 81.6 | 83.8 | 85.6 |
| $C_4H_{10}O$ | $CH_3O\cdot$ | $nC_3H_7\cdot$ | 84.8 | 81.4 | 83.6 | 85.4 |
| $C_5H_{12}O$ | $CH_3O\cdot$ | $C_4H_9\cdot$ | 81.8 | 81.2 | 83.5 | 85.0 |
| $C_4H_{10}O$ | $C_2H_5O\cdot$ | $C_2H_5\cdot$ | 84.9 | 85.4 | 87.6 | 89.2 |

| | | | | | | |
|---|---|---|---|---|---|---|
| $C_4H_8O$ | $C_2H_5O\cdot$ | $C_2H_3\cdot$ | 101.6 | 106.0 | 104.2 | 109.9 |
| $CH_3NO$ | $NO\cdot$ | $CH_3\cdot$ | 41.1 | 38.1 | 40.7 | 44.5 |
| $CH_3N_3$ | $N_3\cdot$ | $CH_3\cdot$ | 80.1 | 70.6 | 73.2 | 77.4 |
| $CH_5N$ | $NH_2\cdot$ | $CH_3\cdot$ | 85.7 | 85.9 | 88.4 | 90.0 |
| $C_2H_7N$ | $NH_2\cdot$ | $C_2H_5\cdot$ | 84.8 | 84.4 | 86.8 | 88.3 |
| $C_2H_3N$ | $CN\cdot$ | $CH_3\cdot$ | 101.5 | 103.0 | 105.4 | 105.5 |
| $CH_2N_2$ | $CN\cdot$ | $NH_2\cdot$ | 118.8 | 121.5 | 124.5 | 125.0 |
| $C_6H_{14}$ | $CH_3\cdot$ | $C_5H_{11}\cdot$ | 94.8 | 83.5 | 85.8 | 86.7 |
| $C_6H_{14}$ | $C_3H_7\cdot$ | $C_3H_7\cdot$ | 93.9 | 80.0 | 82.5 | 82.6 |
| $C_6H_{14}$ | $C_2H_5\cdot$ | $C_4H_9\cdot$ | 91.9 | 75.5 | 77.6 | 78.4 |
| $C_6H_{14}$ | $C_3H_7\cdot$ | $C_3H_7\cdot$ | 91.0 | 74.5 | 76.5 | 76.9 |
| $C_7H_{16}$ | $C_3H_7\cdot$ | $C_4H_9\cdot$ | 95.6 | 83.5 | 86.2 | 86.6 |
| $C_7H_{16}$ | $C_3H_7\cdot$ | $C_4H_9\cdot$ | 93.9 | 79.9 | 82.5 | 82.2 |
| $C_7H_{16}$ | $C_3H_7\cdot$ | $C_4H_9\cdot$ | 93.5 | 78.9 | 81.4 | 81.8 |
| $C_7H_{16}$ | $C_3H_7\cdot$ | $C_4H_9\cdot$ | 92.5 | 75.3 | 77.8 | 78.0 |
| $C_7H_{16}$ | $C_3H_7\cdot$ | $C_4H_9\cdot$ | 88.9 | 68.7 | 70.8 | 71.2 |
| $C_8H_{18}$ | $C_3H_7\cdot$ | $C_5H_{11}\cdot$ | 90.8 | 72.9 | 75.1 | 75.5 |
| | MAD | | | 5.8 | 5.3 | 5.8 |

2. BDE99 set

| Species | Radical 1 | Radical 2 | Ref [3] | B3LYP | ML-B3LYP-g | ML-B3LYP-p |
|---|---|---|---|---|---|---|
| FOOF | F | $FO_2$ | -17.7 | -16.9 | -18.7 | -27.0 |
| FOOF | OF | | -46.2 | -42.2 | -44.6 | -50.5 |
| OCLO | O | ClO | -62.7 | -58.0 | -59.5 | -61.0 |
| CLOO | CLO | O | -60.9 | -60.6 | -62.2 | -64.7 |
| CLOO | CL | $O_2$ | -5.6 | -3.2 | -5.3 | -13.2 |
| $FO_2$ | OF | O | -81.6 | -80.0 | -81.9 | -81.9 |
| $FO_2$ | F | $O_2$ | -13.9 | -11.8 | -14.1 | -22.5 |
| $CL_2O$ | CLO | Cl | -36.0 | -29.9 | -33.1 | -39.6 |
| $F_2O$ | OF | F | -40.7 | -37.5 | -39.5 | -46.2 |
| HOCL | H | ClO | -100.8 | -95.9 | -97.8 | -101.3 |
| HOCL | OH | Cl | -59.0 | -54.1 | -56.7 | -60.6 |
| HOF | H | OF | -105.6 | -100.8 | -102.3 | -104.2 |
| HOF | OH | F | -51.5 | -48.4 | -50.3 | -55.6 |
| $NO_2$ | NO | O | -75.1 | -77.1 | -78.9 | -80.2 |
| $N_2O$ | NO | N | -118.1 | -120.0 | -124.4 | -123.4 |
| $N_2O$ | $N_2$ | O | -42.4 | -45.8 | -48.0 | -48.8 |
| t-HONO | H | $NO_2$ | -84.8 | -79.8 | -81.4 | -84.2 |
| t-HONO | OH | NO | -52.7 | -49.8 | -52.4 | -57.4 |
| HNC | H | CN | -116.9 | -119.5 | -121.0 | -120.5 |
| HNC | NH | C | -215.1 | -210.3 | -214.1 | -213.4 |

| | | | | | | |
|---|---|---|---|---|---|---|
| HONC | OH | CN | -61.6 | -62.7 | -65.2 | -66.8 |
| HNCO | NH | CO | -91.9 | -94.1 | -96.9 | -95.4 |
| HCNO | CH | NO | -128.0 | -128.2 | -131.7 | -134.8 |
| HNO | H | NO | -53.1 | -50.8 | -52.6 | -55.6 |
| HNO | NH | O | -122.8 | -117.3 | -120.8 | -122.0 |
| methanol | $CH_3$ | OH | -98.4 | -92.9 | -95.1 | -96.4 |
| t-HCOH | CH | OH | -131.1 | -126.8 | -128.9 | -131.3 |
| t-HCOH | HCO | H | -43.1 | -39.8 | -41.3 | -43.5 |
| formic | HCO | OH | -115.3 | -109.5 | -112.0 | -114.8 |
| ketene | $CH_2C$ | O | -173.5 | -173.2 | -175.0 | -175.3 |
| ketene | $CH_2$-trip | CO | -83.0 | -85.9 | -88.1 | -85.6 |
| glyoxal | HCO | | -76.3 | -69.6 | -72.4 | -77.0 |
| acetaldehyde | $CH_3$ | HCO | -90.6 | -84.8 | -87.3 | -90.4 |
| $F_2CO$ | $CF_2$ | O | -161.9 | -159.2 | -161.1 | -160.5 |
| HCOF | HCO | F | -124.3 | -120.0 | -122.2 | -126.1 |
| $H_2CO$ | HCO | H | -95.2 | -92.8 | -94.5 | -96.1 |
| $H_2CO$ | $CH_2$-trip | O | -183.9 | -180.3 | -183.5 | -181.0 |
| HCO | H | CO | -19.7 | -25.0 | -24.5 | -21.5 |
| HCO | CH | O | -195.2 | -194.1 | -195.6 | -194.8 |
| $CS_2$ | CS | S | -108.6 | -110.2 | -112.3 | -113.2 |
| $CO_2$ | CO | O | -130.4 | -131.8 | -133.9 | -133.3 |
| $CH_2NH_2$ | $CH_2$-trip | $NH_2$ | -108.9 | -106.9 | -108.5 | -105.5 |
| $CH_2NH_2$ | $CH_2NH$ | H | -42.8 | -45.3 | -44.2 | -42.6 |
| $CH_3NH$ | $CH_3$ | NH | -83.7 | -81.5 | -83.3 | -81.9 |
| $CH_3NH$ | $CH_2NH$ | H | -35.2 | -38.2 | -37.2 | -36.0 |
| $CH_3NH_2$ | $CH_2NH_2$ | H | -100.0 | -96.4 | -98.2 | -99.6 |
| $CH_3NH_2$ | $CH_3NH$ | H | -107.7 | -103.5 | -105.2 | -106.1 |
| $CH_2NH$ | HCNH | H | -103.2 | -100.2 | -102.0 | -103.5 |
| HCNH | NH | CH | -168.9 | -167.1 | -169.1 | -167.3 |
| HCNH | HCN | H | -22.8 | -27.6 | -26.6 | -24.2 |
| HCN | CN | H | -132.1 | -133.5 | -135.3 | -134.5 |
| HCN | CH | N | -229.2 | -226.7 | -230.5 | -226.8 |
| NCCN | CN | | -139.3 | -144.3 | -147.4 | -146.8 |
| $H_2S$ | HS | H | -96.2 | -93.5 | -94.6 | -96.3 |
| t-HOOO | HOO | O | -57.8 | -56.3 | -57.9 | -59.7 |
| t-HOOO | OH | $O_2$ | -5.3 | -2.3 | -4.2 | -12.5 |
| t-HOOO | H | $O_3$ | -85.9 | -93.7 | -92.7 | -88.0 |
| $O_3$ | $O_2$ | O | -26.6 | -15.6 | -19.5 | -31.4 |
| HOOH | HOO | H | -93.6 | -88.3 | -89.9 | -92.2 |
| HOOH | OH | | -54.7 | -50.0 | -52.1 | -55.8 |
| SSH | HS | S | -77.4 | -74.7 | -76.5 | -74.6 |

| | | | | | | |
|---|---|---|---|---|---|---|
| SSH | $S_2$ | H | -60.9 | -59.7 | -61.0 | -65.1 |
| HOO | OH | O | -68.3 | -68.8 | -70.1 | -70.6 |
| HOO | $O_2$ | H | -54.7 | -53.1 | -54.3 | -59.7 |
| $H_2O$ | OH | H | -125.8 | -121.7 | -123.0 | -123.9 |
| HNNN | $N_2$ | NH | -20.2 | -23.9 | -26.3 | -26.0 |
| $N_2H_4$ | $NH_2$ | | -73.1 | -67.5 | -70.3 | -72.4 |
| t-$N_2H_2$ | NH | | -130.3 | -124.3 | -128.3 | -127.5 |
| $N_2H$ | NH | N | -141.8 | -143.5 | -146.4 | -138.1 |
| $NH_2Cl$ | $NH_2$ | Cl | -65.5 | -60.0 | -62.9 | -66.6 |
| $NH_3$ | $NH_2$ | H | -115.4 | -112.3 | -114.0 | -114.7 |
| $NH_2$ | NH | H | -99.5 | -99.1 | -100.1 | -98.1 |
| allene | $CH_2C$ | $CH_2$-trip | -153.4 | -152.0 | -154.1 | -151.7 |
| propyne | CCH | $CH_3$ | -131.6 | -129.6 | -131.9 | -130.2 |
| propene | $CH_2CH$ | $CH_3$ | -107.6 | -101.1 | -103.4 | -104.3 |
| $C_2H_3F$ | $CH_2CH$ | F | -127.8 | -124.1 | -126.2 | -127.5 |
| $C_2H_6$ | $CH_3$ | | -97.3 | -91.4 | -93.6 | -95.3 |
| $C_2H_4$ | $CH_2$-trip | | -182.6 | -178.2 | -181.6 | -176.6 |
| $CH_2CH$ | $CH_2C$ | H | -86.2 | -87.4 | -87.0 | -86.5 |
| $CH_2CH$ | $C_2H_2$ | H | -40.6 | -44.3 | -43.5 | -43.7 |
| $CH_2C$ | $CH_2$-trip | C | -169.2 | -166.7 | -170.2 | -167.8 |
| HCCF | CCH | F | -132.3 | -132.7 | -134.7 | -133.8 |
| HCCF | CH | CF | -181.5 | -176.1 | -179.2 | -181.2 |
| $C_2H_2$ | CCH | H | -139.4 | -140.0 | -141.5 | -138.2 |
| $C_2H_2$ | CH | | -237.1 | -231.4 | -234.4 | -236.3 |
| $CH_3F$ | $CH_3$ | F | -115.1 | -111.6 | -113.6 | -115.4 |
| $CH_4$ | $CH_3$ | H | -112.6 | -110.6 | -112.0 | -112.2 |
| $CH_3$ | $CH_2$-trip | H | -117.1 | -117.3 | -118.3 | -115.1 |
| $CH_2$-trip | CH | H | -106.5 | -106.5 | -106.7 | -109.9 |
| $CF_2$ | CF | F | -126.1 | -121.0 | -123.0 | -126.7 |
| CLCN | CN | Cl | -104.1 | -103.3 | -106.5 | -109.2 |
| $B_2H_6$ | $BH_3$ | | -44.5 | -39.5 | -39.6 | -41.1 |
| $S_2O$ | $S_2$ | O | -104.5 | -95.7 | -99.2 | -108.6 |
| $S_2O$ | S | SO | -82.3 | -72.9 | -77.0 | -84.6 |
| $SO_3$ | $SO_2$ | O | -86.3 | -80.2 | -82.2 | -82.2 |
| $SO_2$ | SO | O | -134.2 | -123.2 | -127.2 | -132.5 |
| $S_4$-C2V | $S_3$ | S | -66.0 | -59.6 | -61.3 | -62.7 |
| $S_4$-C2V | $S_2$ | | -25.9 | -12.5 | -16.0 | -35.5 |
| $P_4$ | $P_2$ | | -55.4 | -47.8 | -48.0 | -43.3 |
| | MAD | | | 3.7 | 2.6 | 2.8 |

TABLE S5: Computational results in TEST12 database, part E: BH

1. HTBH38 set

| Formula | Direction | Ref [6, 7] | B3LYP | ML-B3LYP-g | ML-B3LYP-p |
|---|---|---|---|---|---|
| $H + HCl \longrightarrow H_2 + Cl$ | $V_f^{\neq}$ | 5.7 | -1.0 | 0.4 | 4.7 |
| | $V_r^{\neq}$ | 7.9 | 4.5 | 4.6 | 6.3 |
| $OH + H_2 \longrightarrow H_2O + H$ | $V_f^{\neq}$ | 4.9 | 1.0 | 1.1 | 2.7 |
| | $V_r^{\neq}$ | 21.2 | 12.6 | 13.4 | 16.7 |
| $CH_3 + H_2 \longrightarrow CH_4 + H$ | $V_f^{\neq}$ | 12.1 | 8.9 | 8.9 | 10.2 |
| | $V_r^{\neq}$ | 15.3 | 9.4 | 10.3 | 12.5 |
| $OH + CH_4 \longrightarrow H_2O + CH_3$ | $V_f^{\neq}$ | 6.5 | 2.5 | 3.1 | 3.9 |
| | $V_r^{\neq}$ | 19.6 | 13.6 | 14.1 | 15.5 |
| $H + H_2 \longrightarrow H_2 + H$ | $V_f^{\neq}$ | 9.6 | 4.1 | 4.3 | 7.1 |
| | $V_r^{\neq}$ | 9.6 | 4.1 | 4.3 | 7.1 |
| $OH + NH_3 \longrightarrow H_2O + NH_2$ | $V_f^{\neq}$ | 3.0 | -2.2 | -1.3 | -0.1 |
| | $V_r^{\neq}$ | 12.7 | 7.2 | 7.7 | 9.2 |
| $HCL + CH_3 \longrightarrow CH_4 + Cl$ | $V_f^{\neq}$ | 1.7 | -1.3 | -0.6 | 1.0 |
| | $V_r^{\neq}$ | 7.1 | 4.7 | 4.9 | 4.8 |
| $OH + C_2H_6 \longrightarrow H_2O + C_2H_5$ | $V_f^{\neq}$ | 3.2 | -0.4 | 0.2 | 0.8 |
| | $V_r^{\neq}$ | 19.9 | 15.2 | 15.7 | 17.2 |
| $F + H_2 \longrightarrow HF + H$ | $V_f^{\neq}$ | 1.4 | -5.4 | -5.3 | -3.5 |
| | $V_r^{\neq}$ | 33.4 | 22.5 | 23.2 | 27.5 |
| $O + CH_4 \longrightarrow OH + CH_3$ | $V_f^{\neq}$ | 13.5 | 7.7 | 8.5 | 10.5 |
| | $V_r^{\neq}$ | 7.9 | 4.2 | 4.4 | 5.2 |
| $H + PH_3 \longrightarrow H_2 + PH_2$ | $V_f^{\neq}$ | 3.1 | -1.1 | -1.0 | 0.4 |
| | $V_r^{\neq}$ | 23.2 | 23.1 | 23.3 | 23.3 |
| $H + HO \longrightarrow H_2 + O$ | $V_f^{\neq}$ | 10.5 | 3.5 | 3.9 | 6.3 |
| | $V_r^{\neq}$ | 12.9 | 6.5 | 6.6 | 9.4 |
| $H + H_2S \longrightarrow H_2 + HS$ | $V_f^{\neq}$ | 3.5 | -0.6 | -0.4 | 1.4 |
| | $V_r^{\neq}$ | 16.8 | 16.0 | 15.7 | 15.1 |
| $O + HCL \longrightarrow OH + Cl$ | $V_f^{\neq}$ | 9.6 | 1.6 | 2.7 | 6.3 |
| | $V_r^{\neq}$ | 9.4 | 4.1 | 4.2 | 4.8 |
| $CH_3 + NH_2 \longrightarrow CH_4 + NH$ | $V_f^{\neq}$ | 8.0 | 6.1 | 6.4 | 6.5 |
| | $V_r^{\neq}$ | 22.4 | 17.6 | 18.3 | 20.7 |
| $C_2H_5 + NH_2 \longrightarrow C_2H_6 + NH$ | $V_f^{\neq}$ | 7.5 | 8.1 | 8.5 | 8.4 |
| | $V_r^{\neq}$ | 18.3 | 15.0 | 15.8 | 17.8 |
| $NH_2 + C_2H_6 \longrightarrow NH_3 + C_2H_5$ | $V_f^{\neq}$ | 10.4 | 9.1 | 9.7 | 10.1 |
| | $V_r^{\neq}$ | 17.4 | 15.3 | 16.2 | 17.3 |
| $NH_2 + CH_4 \longrightarrow NH_3 + CH_3$ | $V_f^{\neq}$ | 14.5 | 11.6 | 12.2 | 12.9 |
| | $V_r^{\neq}$ | 17.8 | 13.3 | 14.2 | 15.4 |
| *s-trans cis*-$C_5H_8 \longrightarrow$ | $V_f^{\neq}$ | 38.4 | 38.8 | 39.0 | 36.6 |

| | | | | | |
|---|---|---|---|---|---|
| *s-trans cis*-$C_5H_8$ | $V_r^{\neq}$ | 38.4 | 38.8 | 39.0 | 36.6 |
| MAD | | | 4.3 | 3.9 | 2.4 |

2. NHTBH38 set

| Formula | Direction | Ref [6, 7] | B3LYP | ML-B3LYP-g | ML-B3LYP-p |
|---|---|---|---|---|---|
| $H + N_2O \longrightarrow OH + N_2$ | $V_f^{\neq}$ | 17.1 | 11.6 | 12.4 | 14.0 |
| | $V_r^{\neq}$ | 82.3 | 72.9 | 72.4 | 72.2 |
| $H + FH \longrightarrow HF + H$ | $V_f^{\neq}$ | 42.2 | 31.0 | 31.0 | 31.3 |
| | $V_r^{\neq}$ | 42.2 | 31.0 | 31.0 | 31.3 |
| $H + ClH \longrightarrow HCl + H$ | $V_f^{\neq}$ | 18.0 | 12.3 | 12.7 | 13.6 |
| | $V_r^{\neq}$ | 18.0 | 12.3 | 12.7 | 13.6 |
| $H + FCH_3 \longrightarrow HF + CH_3$ | $V_f^{\neq}$ | 30.4 | 21.8 | 22.3 | 22.8 |
| | $V_r^{\neq}$ | 57.0 | 48.1 | 47.9 | 48.4 |
| $H + F_2 \longrightarrow HF + F$ | $V_f^{\neq}$ | 2.3 | -7.1 | -6.9 | -4.7 |
| | $V_r^{\neq}$ | 105.8 | 94.6 | 94.1 | 90.7 |
| $CH_3 + FCl \longrightarrow CH_3F + Cl$ | $V_f^{\neq}$ | 6.8 | -0.9 | -0.3 | 2.5 |
| | $V_r^{\neq}$ | 59.2 | 50.9 | 51.1 | 51.2 |
| $F^- + CH_3F \longrightarrow FCH_3 + F^-$ | $V_f^{\neq}$ | -0.3 | -2.0 | -1.9 | -1.4 |
| | $V_r^{\neq}$ | -0.3 | -2.0 | -1.9 | -1.4 |
| $F-\cdots CH_3F \longrightarrow CH_3F\cdots F^-$ | $V_f^{\neq}$ | 13.4 | 10.4 | 10.5 | 10.5 |
| | $V_r^{\neq}$ | 13.4 | 10.4 | 10.5 | 10.5 |
| $Cl^- + CH_3Cl \longrightarrow ClCH_3 + Cl^-$ | $V_f^{\neq}$ | 3.1 | -0.2 | 0.0 | 1.7 |
| | $V_r^{\neq}$ | 3.1 | -0.2 | 0.0 | 1.7 |
| $Cl-\cdots CH_3Cl \longrightarrow ClCH_3\cdots Cl^-$ | $V_f^{\neq}$ | 13.4 | 9.2 | 9.3 | 10.4 |
| | $V_r^{\neq}$ | 13.4 | 9.2 | 9.3 | 10.4 |
| $F^- + CH_3Cl \longrightarrow FCH_3 + Cl^-$ | $V_f^{\neq}$ | -12.5 | -14.3 | -14.2 | -12.9 |
| | $V_r^{\neq}$ | 20.1 | 18.3 | 18.3 | 18.8 |
| $F-\cdots CH_3Cl \longrightarrow FCH_3\cdots Cl^-$ | $V_f^{\neq}$ | 3.4 | 0.6 | 0.7 | 1.3 |
| | $V_r^{\neq}$ | 29.4 | 26.2 | 26.2 | 26.2 |
| $OH^- + CH_3F \longrightarrow HOCH_3 + F^-$ | $V_f^{\neq}$ | -2.4 | -3.9 | -3.9 | -3.2 |
| | $V_r^{\neq}$ | 17.7 | 16.1 | 16.2 | 16.5 |
| $OH-\cdots CH_3F \longrightarrow HOCH_3\cdots F^-$ | $V_f^{\neq}$ | 11.0 | 7.9 | 8.0 | 8.0 |
| | $V_r^{\neq}$ | 47.2 | 45.1 | 45.2 | 45.5 |
| $H + N_2 \longrightarrow HN_2$ | $V_f^{\neq}$ | 14.4 | 7.6 | 8.2 | 10.5 |
| | $V_r^{\neq}$ | 10.6 | 10.3 | 10.0 | 7.5 |
| $H + CO \longrightarrow HCO$ | $V_f^{\neq}$ | 3.2 | -0.7 | -0.3 | 0.6 |
| | $V_r^{\neq}$ | 22.7 | 24.3 | 24.3 | 22.1 |
| $H + C_2H_4 \longrightarrow CH_3CH_2$ | $V_f^{\neq}$ | 1.7 | -0.3 | 0.2 | 1.1 |
| | $V_r^{\neq}$ | 41.8 | 41.6 | 41.4 | 42.5 |
| $CH_3 + C_2H_4 \longrightarrow CH_3CH_2CH_2$ | $V_f^{\neq}$ | 6.9 | 6.1 | 6.6 | 7.5 |
| | $V_r^{\neq}$ | 33.0 | 29.5 | 30.0 | 32.7 |

| | | | | | |
|---|---|---|---|---|---|
| HCN ⟶ HNC | $V_f^{\neq}$ | 48.1 | 47.5 | 47.8 | 46.0 |
| | $V_r^{\neq}$ | 32.8 | 33.4 | 33.5 | 32.0 |
| MAD | | | 4.4 | 4.2 | 3.7 |

## II. COMPUTATIONAL RESULTS IN GMTKN55 DATABASE

MAD of B3LYP, ML-B3LYP-g, and ML-B3LYP-p methods with and without DFT-D4 correction across various subsets in the GMTKN55 database are summarized in Tables table S6. All energy values are reported in kcal/mol.

TABLE S6: MAD in GMTKN55 datebase [8–10]

1. Basic properties and reaction energies for small systems

| dataset | B3LYP | B3LYP+D4 | ML-B3LYP-g | ML-B3LYP-g+D4 | ML-B3LYP-p | ML-B3LYP-p+D4 |
|---|---|---|---|---|---|---|
| W4_11 | 4.49 | 3.51 | 3.70 | 4.04 | 3.09 | 3.35 |
| G21EA | 3.84 | 3.55 | 3.68 | 3.69 | 3.39 | 3.34 |
| G21IP | 3.56 | 3.50 | 3.33 | 3.32 | 3.43 | 3.46 |
| DIPCS10 | 4.74 | 4.31 | 4.45 | 4.33 | 4.21 | 4.06 |
| PA26 | 1.97 | 1.69 | 2.06 | 1.77 | 1.71 | 1.63 |
| SIE4x4 | 17.35 | 17.63 | 17.00 | 17.58 | 15.12 | 15.40 |
| ALKBDE10 | 4.07 | 3.88 | 3.70 | 3.70 | 3.26 | 3.06 |
| YBDE18 | 8.59 | 5.00 | 7.78 | 4.98 | 8.05 | 4.54 |
| AL2X6 | 9.10 | 3.44 | 9.03 | 3.44 | 10.23 | 4.57 |
| HEAVYSB11 | 7.94 | 4.25 | 6.59 | 2.89 | 4.84 | 2.09 |
| NBPRC | 5.01 | 1.92 | 4.95 | 1.93 | 4.99 | 2.11 |
| ALK8 | 6.26 | 5.31 | 6.26 | 5.31 | 10.36 | 8.94 |
| RC21 | 2.08 | 2.41 | 2.08 | 2.96 | 2.40 | 1.73 |
| G2RC | 2.86 | 3.05 | 2.82 | 3.68 | 2.88 | 3.50 |
| BH76RC | 2.11 | 2.08 | 2.11 | 2.08 | 1.46 | 1.54 |
| FH51 | 4.01 | 2.72 | 4.01 | 2.73 | 3.88 | 2.66 |
| TAUT15 | 1.18 | 1.17 | 1.16 | 1.49 | 0.99 | 0.98 |
| DC13 | 14.73 | 9.13 | 14.21 | 9.12 | 11.89 | 8.79 |

2. Reaction energies for large systems and isomerisation reactions

| dataset | B3LYP | B3LYP+D4 | ML-B3LYP-g | ML-B3LYP-g+D4 | ML-B3LYP-p | ML-B3LYP-p+D4 |
|---|---|---|---|---|---|---|
| MB16_43 | 61.40 | 31.56 | 58.30 | 28.80 | 56.11 | 26.71 |
| DARC | 15.22 | 7.38 | 15.26 | 7.38 | 11.59 | 3.93 |
| RSE43 | 1.96 | 1.78 | 1.81 | 1.77 | 1.31 | 1.17 |
| BSR36 | 11.21 | 3.01 | 11.21 | 3.01 | 10.94 | 2.73 |
| CDIE20 | 1.29 | 1.11 | 1.31 | 1.14 | 1.41 | 1.22 |

| | | | | | | |
|---|---|---|---|---|---|---|
| ISO34 | 2.36 | 1.87 | 2.35 | 1.88 | 1.84 | 1.29 |
| ISOL24 | 9.41 | 5.34 | 9.42 | 5.36 | 7.58 | 3.52 |
| C60ISO | 2.10 | 2.78 | 2.12 | 2.79 | 2.57 | 3.54 |
| PArel | 1.08 | 1.05 | 1.09 | 1.05 | 1.01 | 0.97 |

3. Reaction barrier heights

| dataset | B3LYP | B3LYP+D4 | ML-B3LYP-g | ML-B3LYP-g+D4 | ML-B3LYP-p | ML-B3LYP-p+D4 |
|---|---|---|---|---|---|---|
| BH76 | 4.46 | 5.18 | 4.23 | 5.17 | 3.22 | 3.90 |
| BHPERI | 4.29 | 1.15 | 4.38 | 1.10 | 3.88 | 1.55 |
| BHDIV10 | 2.74 | 3.19 | 2.65 | 3.08 | 3.37 | 3.87 |
| INV24 | 1.93 | 1.02 | 1.90 | 1.02 | 2.12 | 1.16 |
| BHROT27 | 0.40 | 0.41 | 0.43 | 0.80 | 0.29 | 0.30 |
| PX13 | 4.66 | 5.32 | 4.57 | 5.23 | 5.96 | 6.62 |
| WCPT18 | 1.37 | 2.43 | 1.27 | 3.54 | 2.71 | 3.78 |

4. Intermolecular noncovalent interactions

| dataset | B3LYP | B3LYP+D4 | ML-B3LYP-g | ML-B3LYP-g+D4 | ML-B3LYP-p | ML-B3LYP-p+D4 |
|---|---|---|---|---|---|---|
| RG18 | 0.80 | 0.14 | 0.80 | 0.14 | 0.96 | 0.29 |
| ADIM6 | 5.03 | 0.28 | 5.01 | 0.27 | 5.55 | 0.81 |
| S22 | 3.76 | 0.42 | 3.76 | 0.42 | 4.27 | 0.28 |
| S66 | 3.22 | 0.30 | 3.22 | 0.30 | 3.69 | 0.36 |
| HEAVY28 | 1.30 | 0.31 | 1.30 | 0.31 | 1.72 | 0.70 |
| WATER27 | 5.29 | 3.82 | 5.36 | 3.93 | 7.94 | 1.28 |
| CARBHB12 | 0.67 | 0.69 | 0.67 | 0.96 | 1.01 | 0.51 |
| PNICO23 | 1.75 | 0.36 | 1.75 | 0.37 | 2.25 | 0.36 |
| HAL59 | 1.72 | 0.51 | 1.71 | 0.50 | 2.15 | 0.41 |
| AHB21 | 0.87 | 0.52 | 0.84 | 0.54 | 1.26 | 0.51 |
| CHB6 | 1.03 | 0.98 | 1.03 | 0.96 | 1.27 | 0.92 |
| IL16 | 4.01 | 0.33 | 3.97 | 0.32 | 4.35 | 0.63 |

5. Intramolecular noncovalent interactions

| dataset | B3LYP | B3LYP+D4 | ML-B3LYP-g | ML-B3LYP-g+D4 | ML-B3LYP-p | ML-B3LYP-p+D4 |
|---|---|---|---|---|---|---|
| IDISP | 16.25 | 3.04 | 16.27 | 3.19 | 15.80 | 2.93 |
| ICONF | 0.58 | 0.28 | 0.59 | 0.29 | 0.63 | 0.29 |
| ACONF | 0.97 | 0.06 | 0.97 | 0.06 | 0.99 | 0.05 |
| Amino20x4 | 0.65 | 0.20 | 0.65 | 0.20 | 0.67 | 0.23 |
| PCONF21 | 3.77 | 0.36 | 3.79 | 0.40 | 3.95 | 0.36 |
| MCONF | 2.49 | 0.26 | 2.47 | 0.27 | 2.67 | 0.26 |
| SCONF | 0.68 | 0.36 | 0.71 | 0.36 | 0.66 | 0.37 |
| UPU23 | 2.42 | 0.98 | 2.42 | 0.98 | 2.55 | 1.04 |

| | | | | | | |
|---|---|---|---|---|---|---|
| BUT14DIOL | 0.40 | 0.48 | 0.39 | 0.46 | 0.45 | 0.42 |

* ghc@everest.hku.hk
† xzheng@fudan.edu.cn

[1] R. Haunschild and W. Klopper, "New accurate reference energies for the G2/97 test set," J. Chem. Phys. **136**, 164102 (2012).

[2] L. A. Curtiss, K. Raghavachari, P. C. Redfern, and J. A. Pople, "Assessment of Gaussian-3 and density functional theories for a larger experimental test set," J. Chem. Phys. **112**, 7374 (2000).

[3] N. Mardirossian and M. Head-Gordon, "Thirty years of density functional theory in computational chemistry: An overview and extensive assessment of 200 density functionals," Mol. Phys. **115**, 2315 (2017).

[4] L. A. Curtiss, P. C. Redfern, K. Raghavachari, and J. A. Pople, "Assessment of Gaussian-2 and density functional theories for the computation of ionization potentials and electron affinities," J. Chem. Phys. **109**, 42 (1998).

[5] Y.-R. Luo, *Handbook of Bond Dissociation Energies in Organic Compounds*, CRC Press, Boca Raton, FL, 2003.

[6] J. Zheng, Y. Zhao, and D. G. Truhlar, "The DBH24/08 database and its use to assess electronic structure model chemistries for chemical reaction barrier heights," J. Chem. Theory Comput. **5**, 808 (2009).

[7] R. Peverati and D. G. Truhlar, "Quest for a universal density functional: The accuracy of density functionals across a broad spectrum of databases in chemistry and physics," Philos. Trans. R. Soc., A **372**, 20120476 (2014).

[8] L. Goerigk, A. Hansen, C. Bauer, S. Ehrlich, A. Najibi, and S. Grimme, "A Look at the Density Functional Theory Zoo with the Advanced GMTKN55 Database for General Main Group Thermochemistry, Kinetics and Noncovalent Interactions," Phys. Chem. Chem. Phys. **19**, 32184 (2017).

[9] E. Caldeweyher, C. Bannwarth, and S. Grimme, "Extension of the D3 Dispersion Coefficient Model," J. Chem. Phys. **147**, 034112 (2017).

[10] E. Caldeweyher, S. Ehlert, A. Hansen, H. Neugebauer, S. Spicher, C. Bannwarth, and S. Grimme, "A Generally Applicable Atomic-Charge Dependent London Dispersion Correction," J. Chem. Phys. **150**, 154122 (2019).
